# Supplementary material for: Guided Image Restoration via Simultaneous Feature and Image Guided Fusion
Source: arXiv:2312.08853 source file (2023-12-14)
Supplement: Supplementary file 1 [file X_suppl.tex]

\clearpage
\setcounter{page}{1}
\maketitlesupplementary


\section{Rationale}
\label{sec:rationale}
% 

\begin{figure*}[t]
	\setlength{\abovecaptionskip}{0.2cm}
	\centering
	% \fbox{\rule{0pt}{2in} \rule{0.9\linewidth}{0pt}}
	\includegraphics[width=1\linewidth]{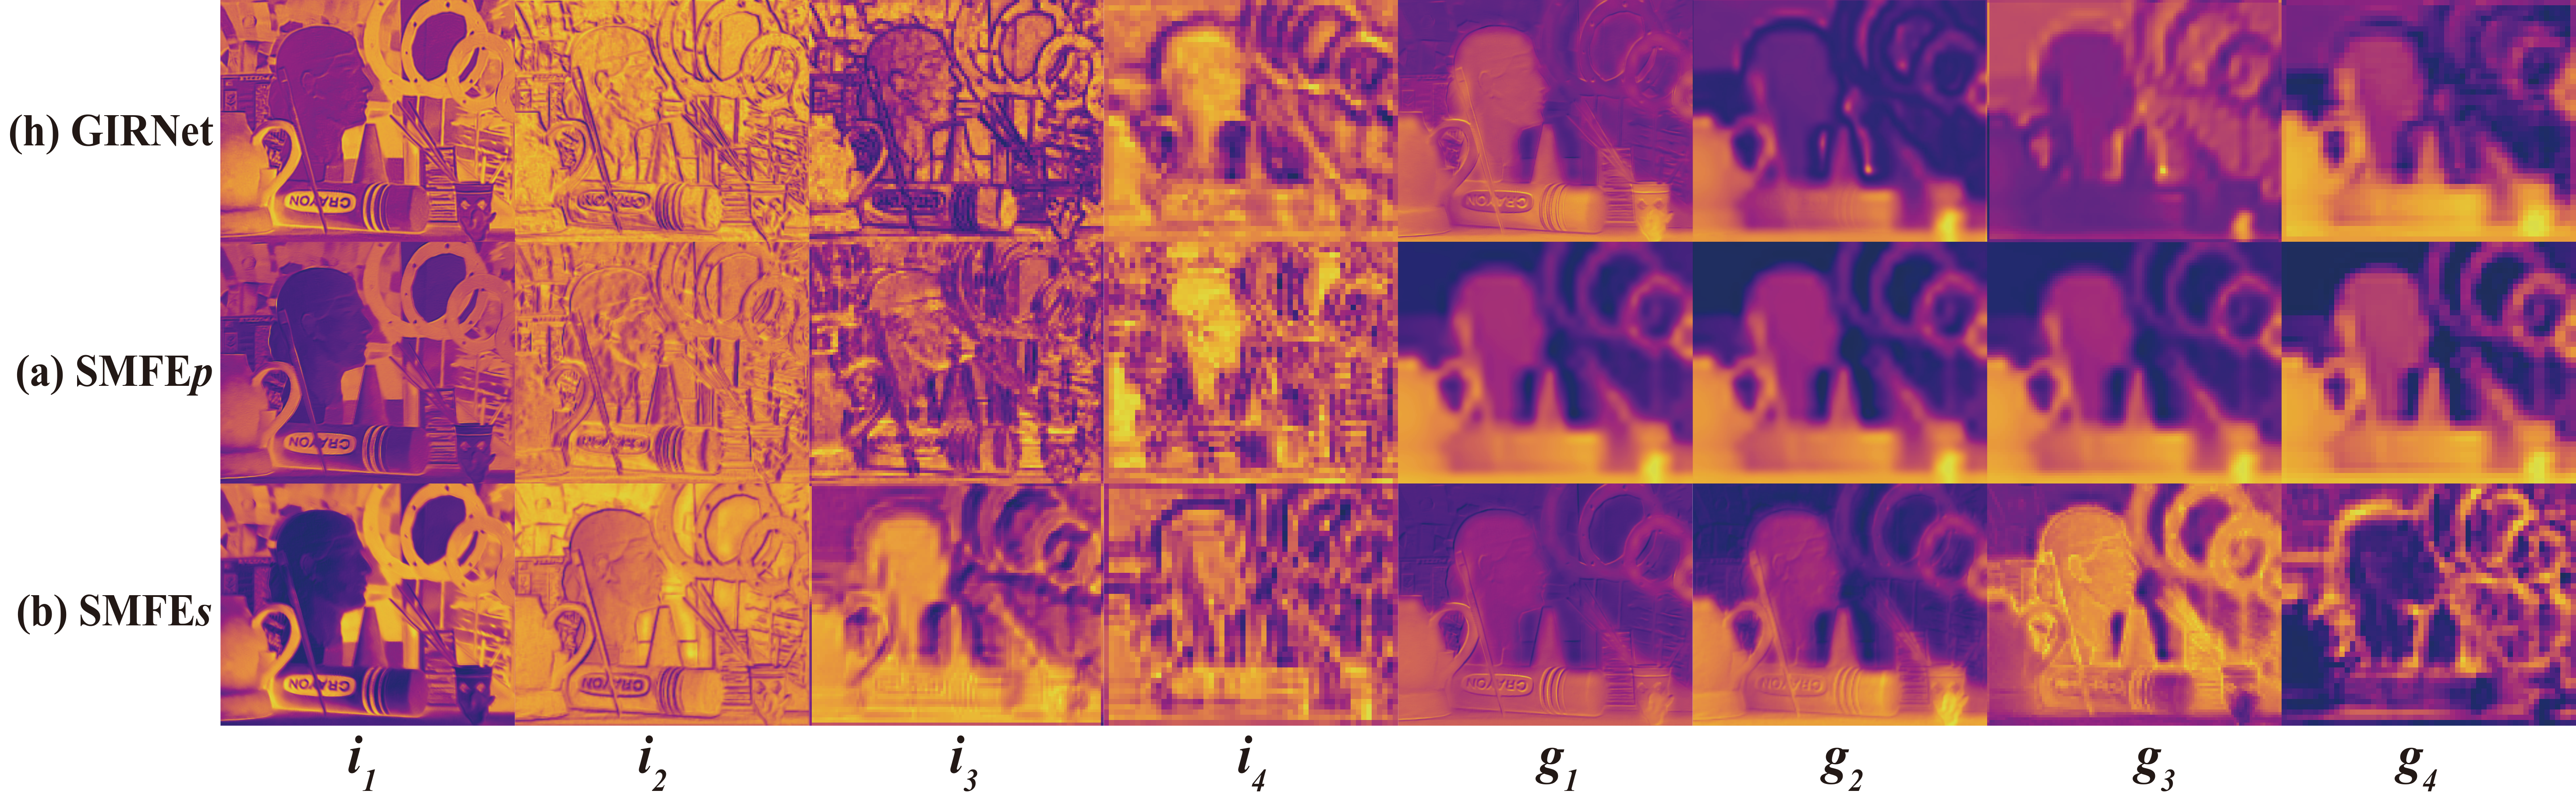}
	%\vspace{-0.5cm}
	\caption{ Visualization of the extracted multi-scaled features by the different SMFE modules.}
	\label{fig:absmfe}
	% \vspace{-0.5cm}
\end{figure*}
\subsection{GIRNet for GDSR}
The GDSR task aims at restoring an HR depth map from an LR one under the guidance of an RGB image captured in the same scene. This is a typical GIR problem, where the LR depth map $P \in \mathbb{R}^{h\times w \times 1}$ is the to-be-restored image, and the HR RGB image $I \in \mathbb{R}^{H\times W \times 3} $ is regarded as the guidance, where $h<H$ and $w<W$. For many deep learning methods, $P$ is generally pre-upsampled, e.g., by bicubic interpolation, to be with the same spatial size of $I$, and we follow this preprocessing way. Then the output should be a reconstructed depth map $Q_{out}\in \mathbb{R}^{H\times W \times 1}$. In this task, we train GIRNet in a supervised way with $L_1$ Loss for 200 epochs, and the initial learning rate is $1\times10^{-4}$ and {\color{red} reduces by 0.2 every 40 steps.}
% \textbf{The number of the base channel in our backbone network is 48.}

% \noindent \textit{a. Experimental Settings}
\subsubsection{Datasets}
We conduct experiments following previous studies \cite{zhao2022dct, zhong2021high}. Specifically, all methods are trained on the first 1000 paired images of the NYU V2 dataset \cite{silberman2012indoor} and tested on the last 449 pairs. In addition, the trained models are also tested on the Middlebury dataset\cite{hirschmuller2007mid} and the Lu \cite{lu2014depth} dataset for evaluating their generalization abilities. For all datasets, we obtain low-resolution depth maps by downsampling the given high-resolution depth maps {\color{red}with the} bicubic interpolation, and consider three SR scales, i.e., 4x, 8x, and 16x.

\subsubsection{Competeting methods and evaluation metrics\label{sec:cm}}
Since our developing goal is a unified model that can be applied to different GIR tasks, we will compare our methods with general-purpose GIR techniques and the methods designed for a specific task. Six representative general purpose methods are considered in all our experiments, including the classical GF \cite{he2010guided, he2012guided}, and five deep learning-based methods, FGF \cite{wu2018fgf}, SVLRM \cite{pan2019spatially}, DKN\cite{kim2021deformable}, CUNet\cite{deng2020cunet}, and DAGF\cite{zhong2021dagif}.
For the GDSR task, we also compare four state-of-the-art specialized deep learning-based approaches, including FDSR \cite{he2021towards}, DCTNet\cite{zhao2022dct},  AHMF \cite{zhong2021high}, and SSDNet \cite{zhao2023spherical}. 
To enable quantitative comparison, we utilize the widely adopted root-mean-square error (RMSE) as the metric to evaluate the performance of all compared methods across all GDSR datasets.

\subsubsection{Experimental Results}

The quantitative results of all the competing methods across all datasets are summarized in Tabel \ref{tab:gdsr}. As can be seen from the table, our proposed approach GIRNet attains the leading performance across all benchmark datasets evaluated, indicating that our proposed method can reconstruct the depth map closest to the ground truth across different scenarios. Besides, considering the average result under each SR scale, our method also consistently performs the best, showing its robustness in
% Specifically, when compared with the generative methods, our method decreases the average RMSE by 0.05 (4x), 0.29 (8x), and 0.62 (16x), and when compared with the second best method SSDNet \cite{zhao2023spherical}, our method decreases the average RMSE by 0.02 (4x), 0.09 (8x), and 0.26 (16x), respectively, suggesting while being generally applicable, 
handling the GDSR task with various degrees of degradation.

It can be seen from Fig.\ref{fig:gdsr} that our qualitative results are also promising. Compared with the methods that are implemented with image level-guided filtering mechanisms, including GF \cite{he2010guided}, FGF \cite{wu2018fgf}, and SVLRM \cite{pan2019spatially}, our method is able to avoid artifacts like ghosting and preserve structures {\color{red}simultaneously}. When competing against other general deep learning-based GIR approaches like FDKN\cite{kim2021deformable}, CUNet \cite{deng2020cunet}, and DAGF \cite{zhong2021dagif}, our method better reconstructs fine texture details. As for the specialized GDSR method, e.g. FDSR \cite{guo2018hierarchical}, AHMF\cite{zhong2021high}, DCTNet\cite{zhao2022dct}, SSDNet \cite{zhao2023spherical}, our method demonstrate superior performance through smooth surfaces and clear depiction of details. These observations show our method effectively overcomes generative methods' limitations of existing general-purpose GIR methods and even outperforms state-of-the-art deep models for the GDSR task.


\begin{figure*}[t]
	\centering
 \captionsetup[subfloat]{labelsep=none,format=plain,labelformat=empty}
	\setlength{\abovecaptionskip}{0.1cm}
	\subfloat[RGB ]{\includegraphics[width=0.14\linewidth]{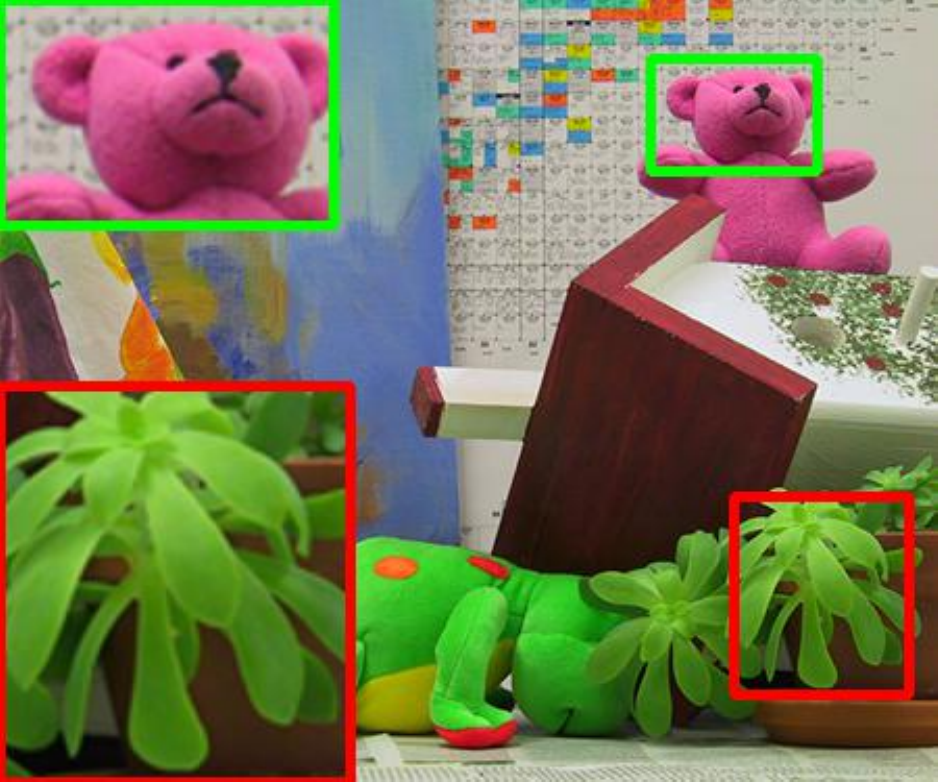}}
	\subfloat[Bicubic (Lr) ]{ \includegraphics[width=0.14\linewidth]{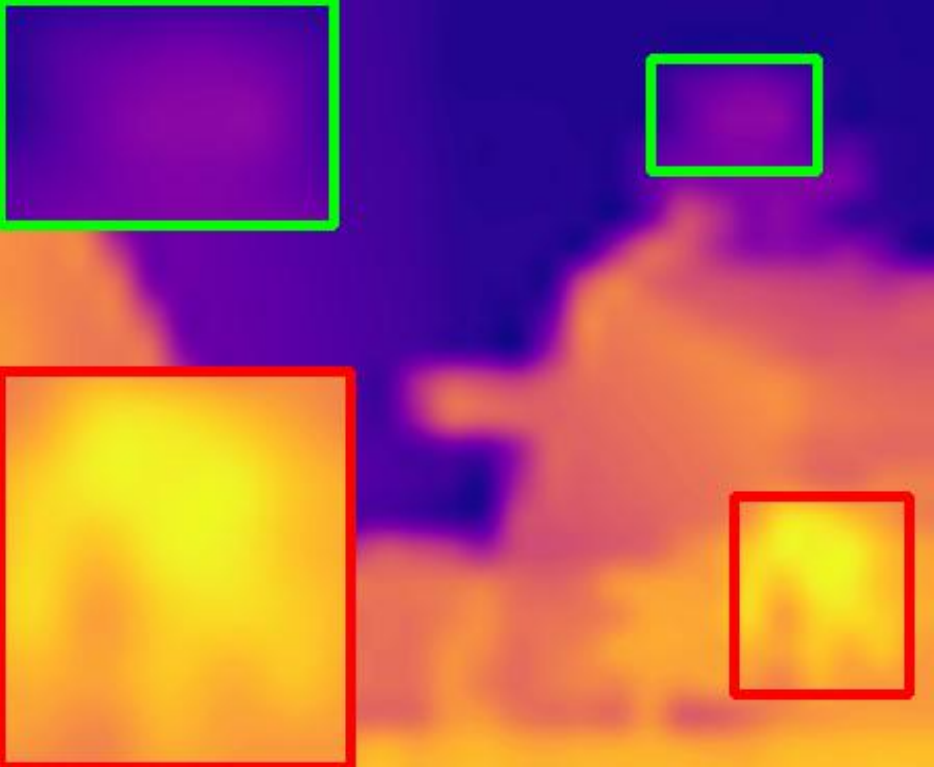}}
	\subfloat[GF]{ \includegraphics[width=0.14\linewidth]{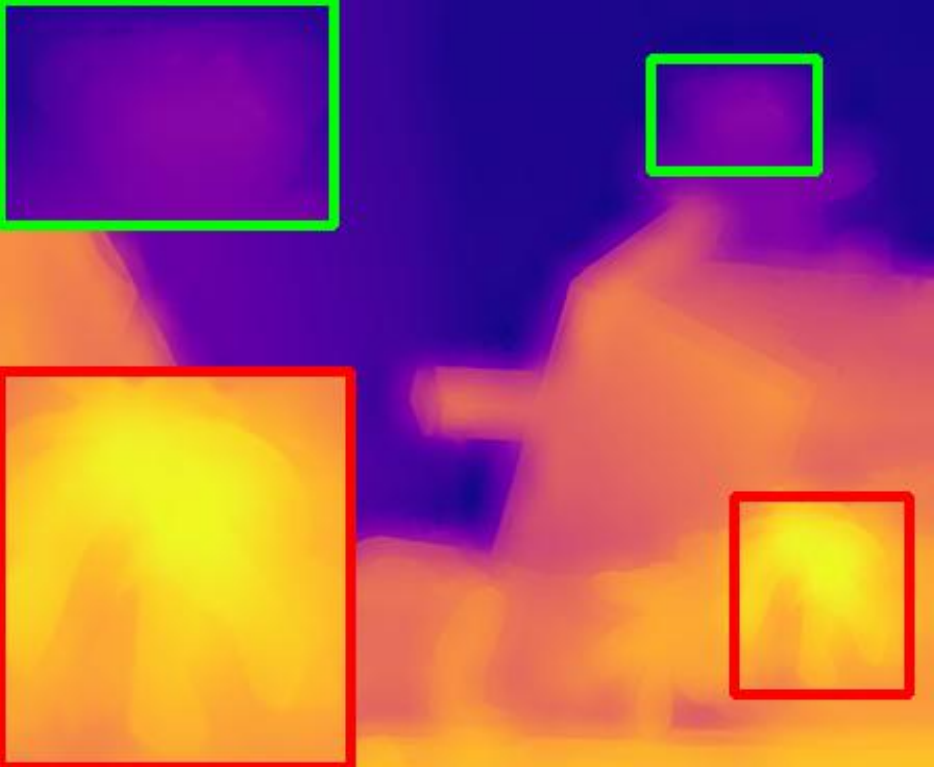}} 
	\subfloat[FGF ]{	\includegraphics[width=0.14\linewidth]{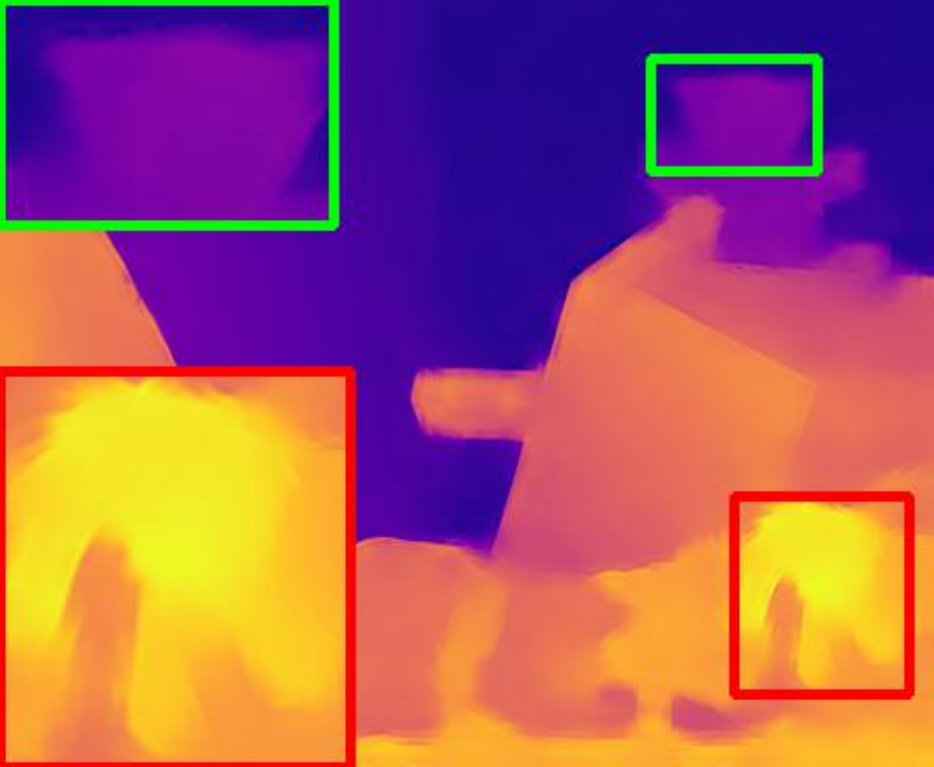}}
	\subfloat[SVLRM ]{ \includegraphics[width=0.14\linewidth]{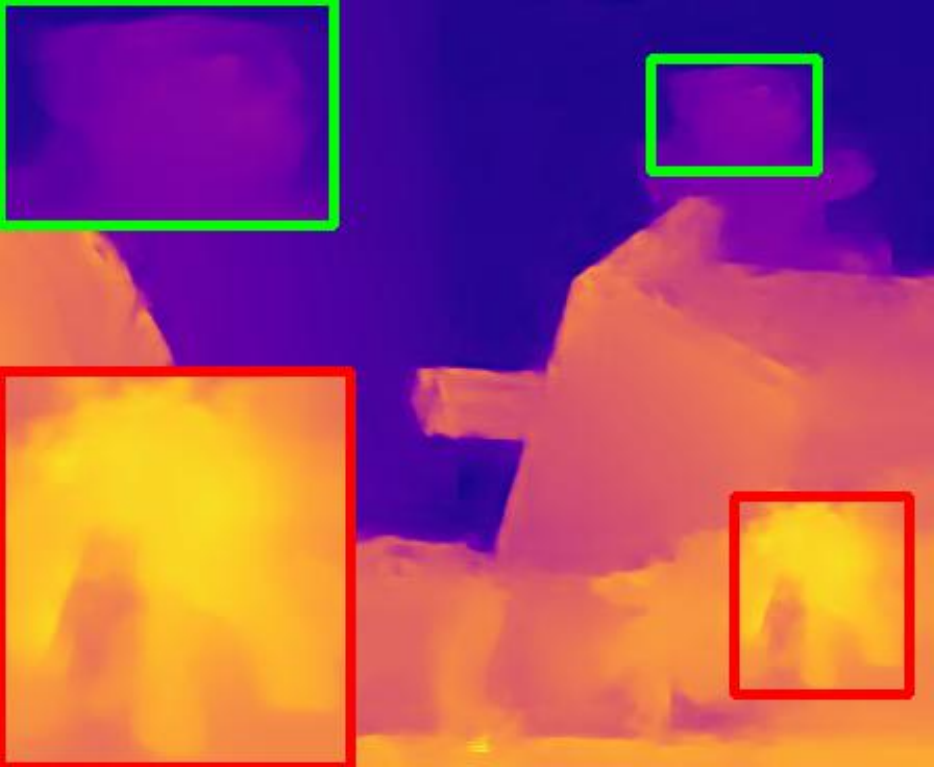}}
	\subfloat[FDKN]{	\includegraphics[width=0.14\linewidth]{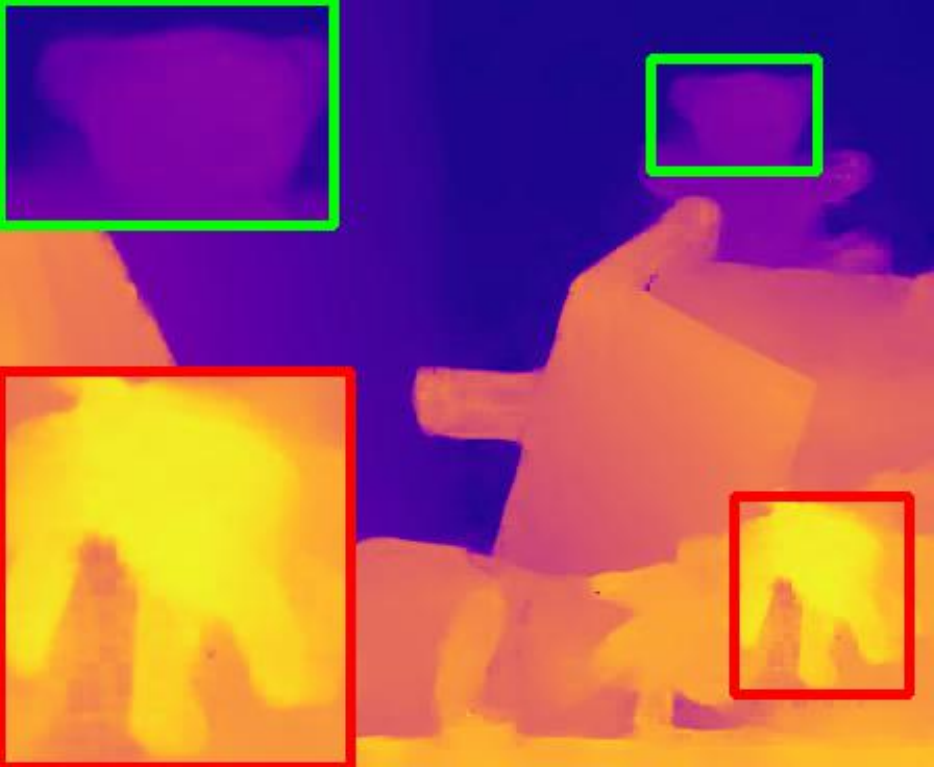}} 
 \subfloat[CUNet]{	\includegraphics[width=0.14\linewidth]{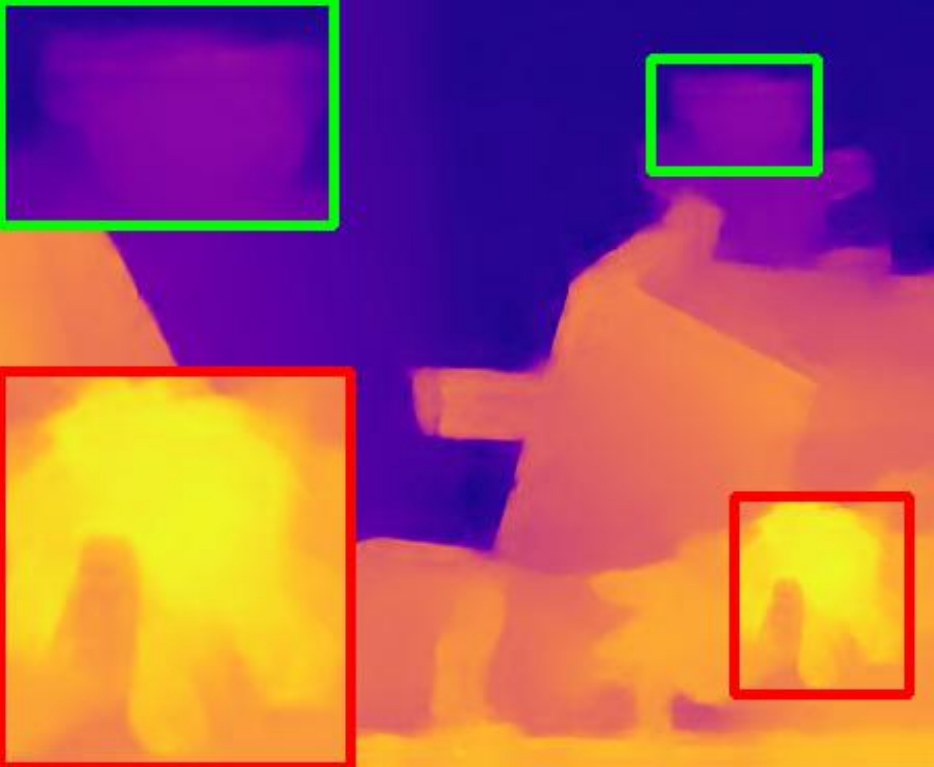}} 
 \\
 % \vspace{-3mm}
 \subfloat[DAGF ]{	\includegraphics[width=0.14\linewidth]{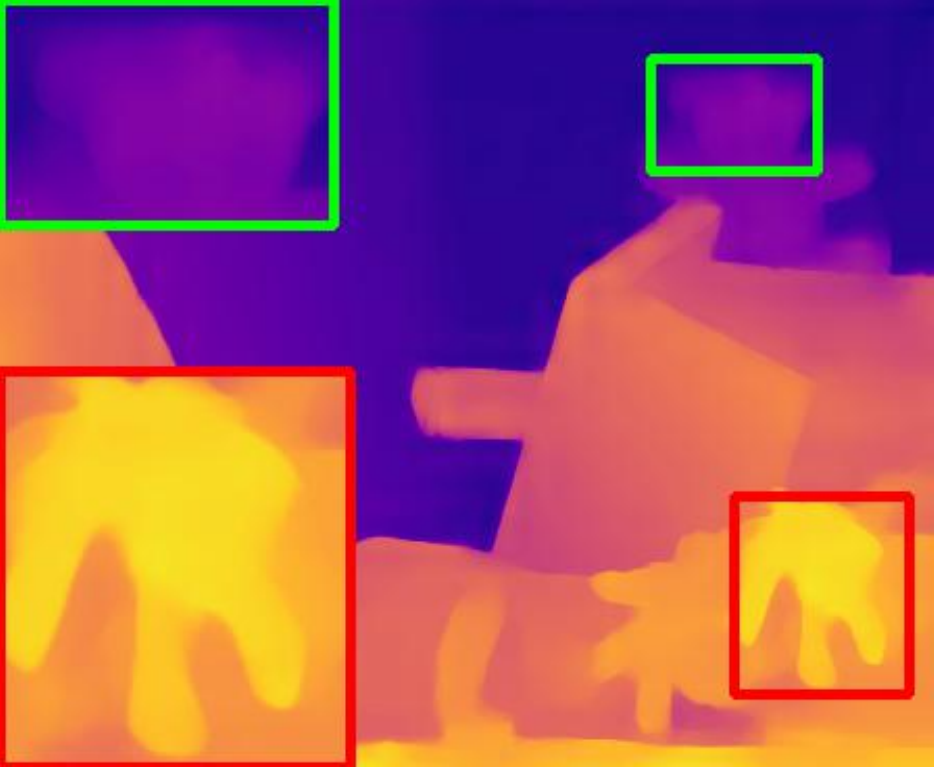}}
 \subfloat[FDSR]{	\includegraphics[width=0.14\linewidth]{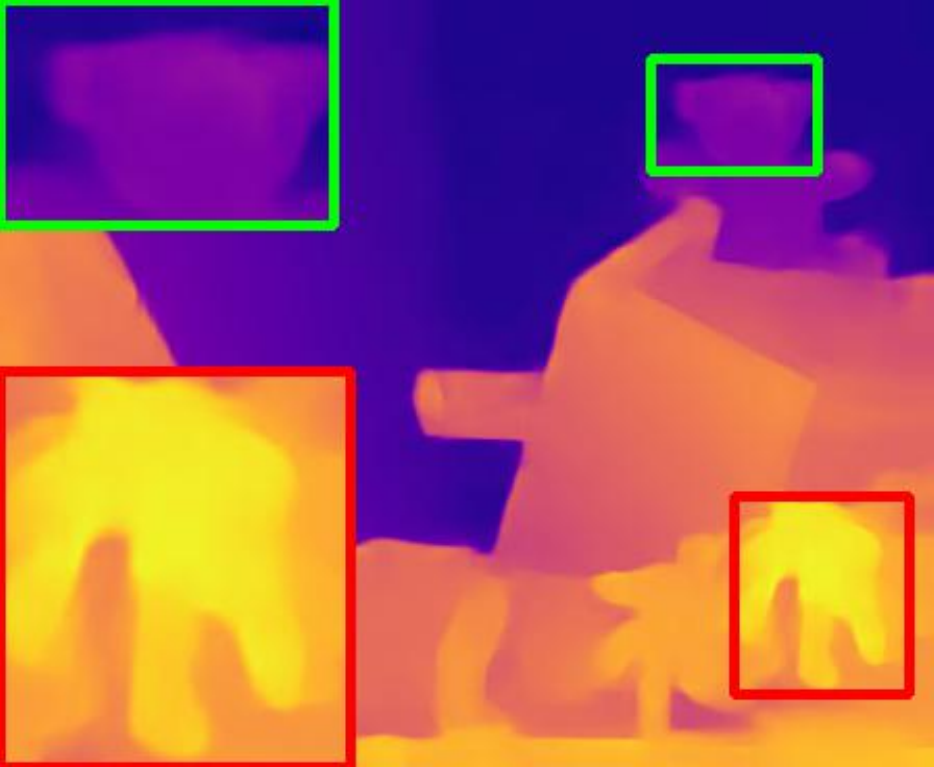}}
 \subfloat[AHMF ]{	\includegraphics[width=0.14\linewidth]{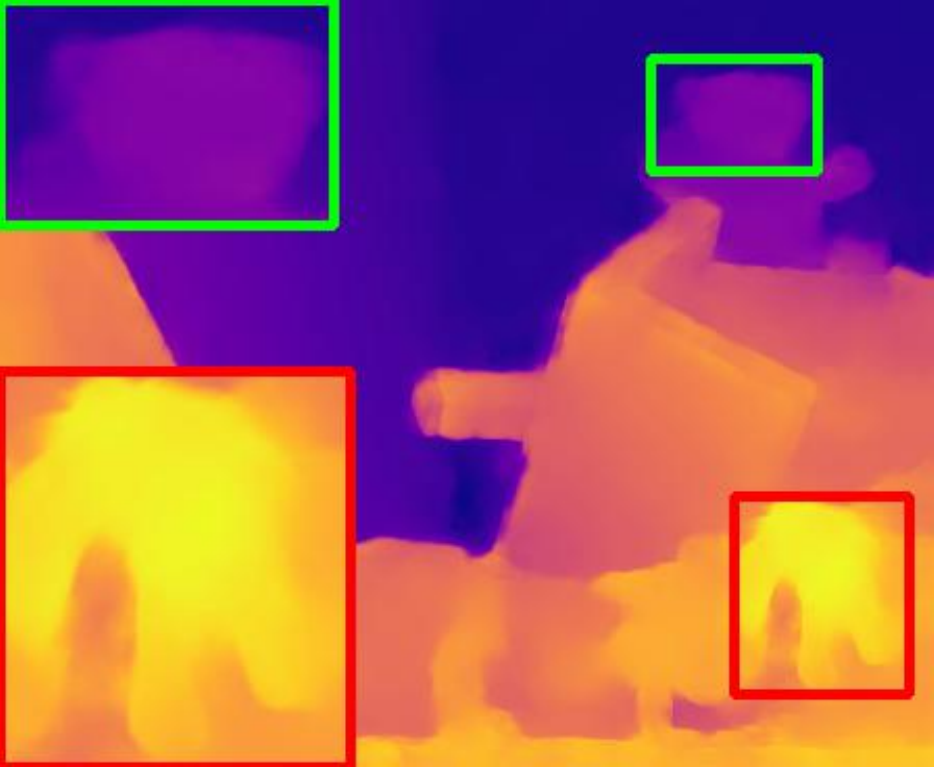}}
 \subfloat[DCTNet ]{	\includegraphics[width=0.14\linewidth]{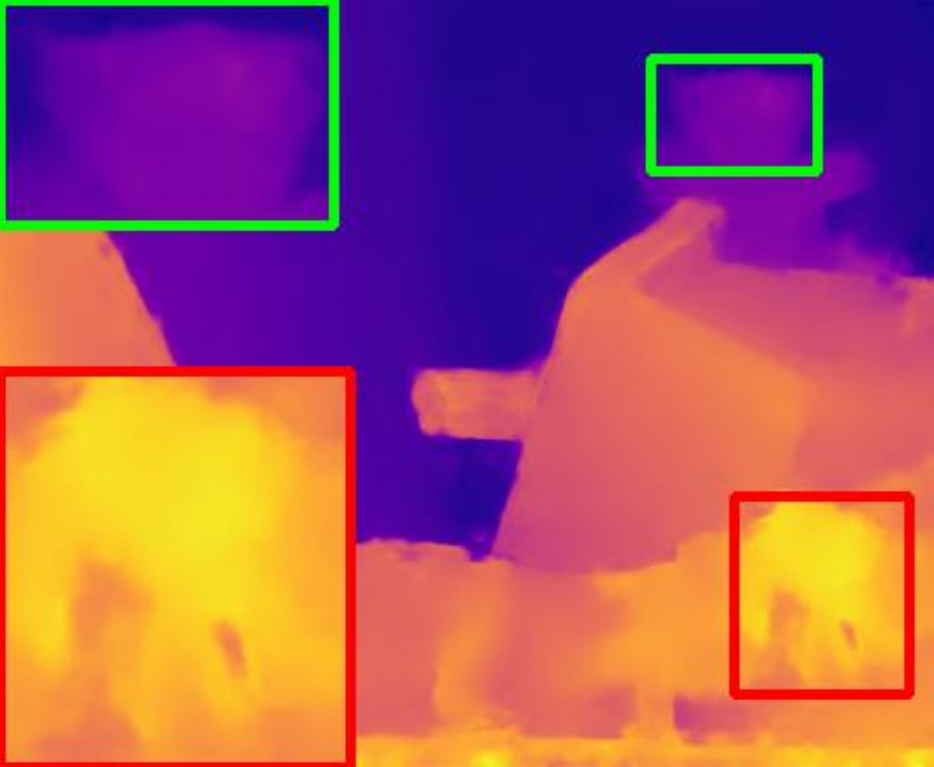}}
 \subfloat[SSDNet ]{	\includegraphics[width=0.14\linewidth]{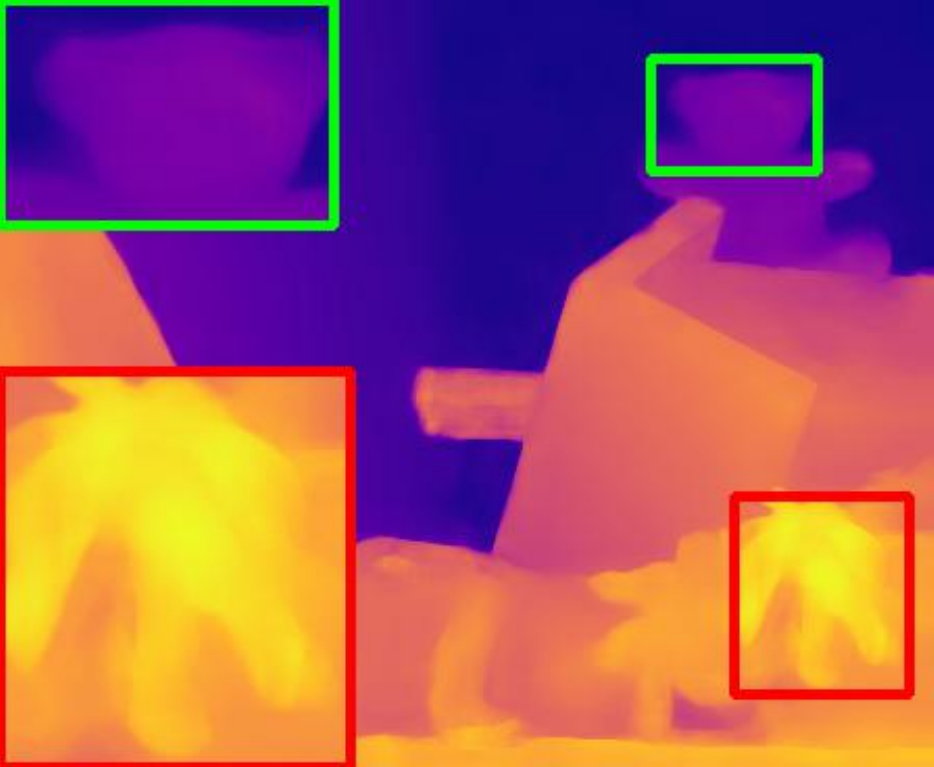}}
 \subfloat[GIRNet]{	\includegraphics[width=0.14\linewidth]{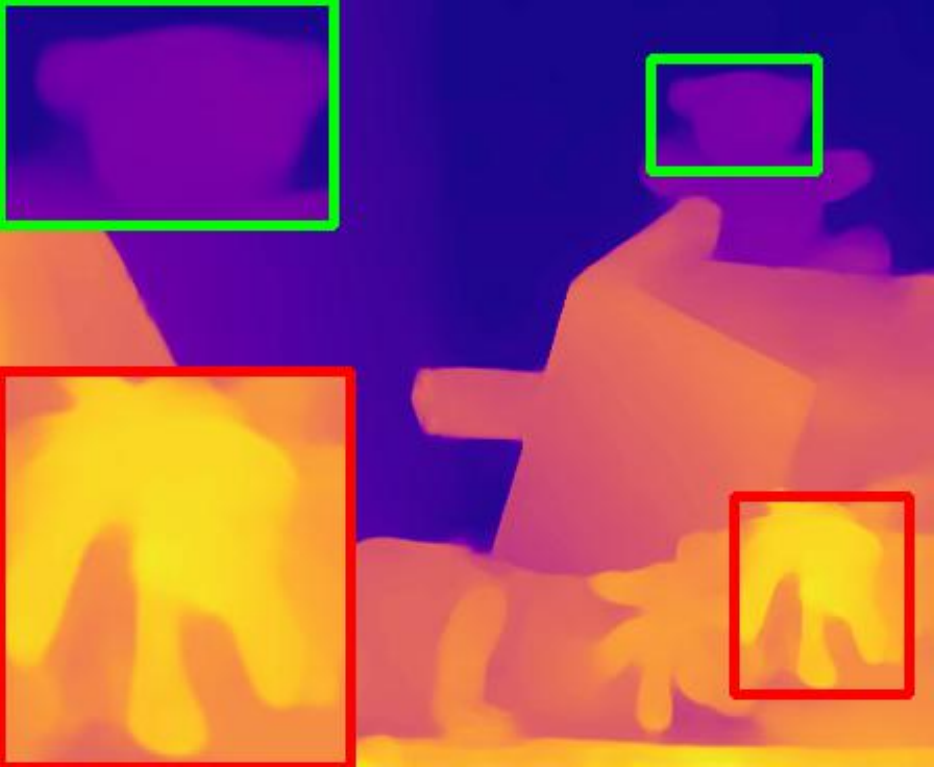}}
  \subfloat[GT]{	\includegraphics[width=0.14\linewidth]{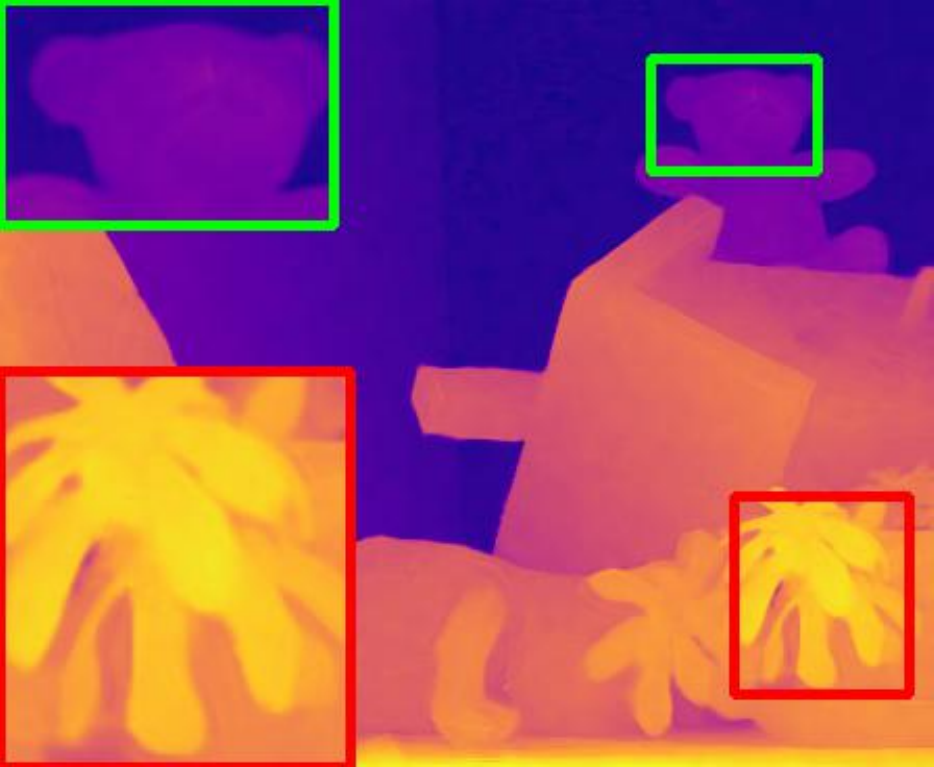}}
	\caption{Visual comparison of competed methods on the 16x Middlebury dataset of the GDSR task. }
	\vspace{-0.5cm}
	\label{fig:gdsr} 
\end{figure*}

\begin{table*}[!ht]
	\centering
	% \setlength{\abovecaptionskip}{0.1cm}
	\caption{Quantitative comparison with the generative and state-of-the-art methods on the GDSR task. We use the RMSE metric (The lower the better). The best performance is shown in bold, and the second is underlined. }
	\begin{tabular}{ccccccccccccc}
		\toprule
		\multirow{2}{*}{Methods}& \multicolumn{3}{c}{Middlebury} & \multicolumn{3}{c}{NYU V2} &  \multicolumn{3}{c}{Lu} & \multicolumn{3}{c}{Average}\\ 
		\cmidrule(lr){2-4}
            \cmidrule(lr){5-7}
            \cmidrule(lr){8-10}
            \cmidrule(lr){11-13}
		~ & 4x & 8x & 16x & 4x & 8x & 16x & 4x & 8x & 16x & 4x & 8x & 16x \\ \hline
 GF\cite{he2010guided}& 3.13 & 4.00 & 6.19 & 5.97 & 7.40 & 11.23 & 4.20 & 5.21 & 7.46 & 4.43  & 5.54  & 8.29   \\
        FGF \cite{wu2018fgf} & 1.36  & 2.28  & 4.34  & 2.39  & 3.82  & 6.98  & 1.37  & 2.35  & 4.61  & 1.71  & 2.82  & 5.31  \\ 
        SVLRM \cite{pan2019spatially} & 1.18 & 2.43 & 5.33 & 1.82 & 3.67 & 7.87 & 1.04 & 2.51 & 6.15 & 1.35  & 2.87  & 6.45   \\ 
        FDKN \cite{kim2021deformable} & 1.09  & 2.09  & 4.27  & 1.64  & 3.30  & 6.62  & \underline{0.79}  & 2.07  & 4.83  & 1.17  & 2.49  & 5.24 \\ 
        CUNet \cite{deng2020cunet}& 1.28 & 2.40 & 4.73 & 2.22 & 4.02 & 7.88 & 1.05 & 2.48 & 5.19 & 1.52  & 2.97  & 5.93   \\ 
        DAGF \cite{zhong2021dagif} & 1.28 & 2.66 & 3.80 & 2.66 & 4.97 & 7.19 & 1.26 & 2.60 & 4.77 & 1.73  & 3.41  & 5.25   \\ \hline
        FDSR \cite{he2021towards} & 1.06 & 2.08 & 4.17 & 1.78 & 3.17 & 5.94 & 1.15 & 2.19 & 5.08 & 1.33  & 2.48  & 5.06   \\ 
        AHMF \cite{zhong2021high} & 1.19 & 2.35 & 4.76 & 1.83 & 3.74 & 7.16 & 0.96 & 2.33 & 5.38 & 1.33  & 2.81  & 5.77   \\
        DCTNet \cite{zhao2022dct} & 1.10& 2.05 & 4.19 & 1.73& 3.56& 6.50 & 0.88& 1.85& 4.39 & 1.24 &2.49 &	5.03 \\ 
        SSDNet \cite{zhao2023spherical} & \underline{1.02} & \underline{1.91} & \underline{4.02} & \textbf{1.60} & \underline{3.14} & \underline{5.86} & 0.80 & \underline{1.82} & \underline{4.77} & \underline{1.14}  & \underline{2.29}  & \underline{4.88}   \\ \hline
        GIRNet (Ours) & \textbf{0.99} & \textbf{1.78} &\textbf{3.46}& \underline{1.63} & \textbf{3.10} & \textbf{5.85} & \textbf{0.74} &\textbf{1.73} & \textbf{4.55} & \textbf{1.12} & \textbf{2.20}  & \textbf{4.62}   \\ \hline
	\end{tabular}
	\label{tab:gdsr}
	% \vspace{-2mm}
\end{table*}
% \begin{table*}[!ht]
% 	\centering
% 	% \setlength{\abovecaptionskip}{0.1cm}
% 	\caption{GDSR }
% 	\begin{tabular}[c]{*{13}{c}}
% 		\toprule
% 		\multirow{2}{*}{Methods}& \multicolumn{3}{c}{Middlebury} & \multicolumn{3}{c}{NYU V2} &  \multicolumn{3}{c}{Lu} &\multicolumn{3}{c}{RGBDD}\\ 
% 		\cmidrule(lr){2-4}
%             \cmidrule(lr){5-7}
%             \cmidrule(lr){8-10}
%             \cmidrule(lr){11-13}
% 		~ & x4 & 8x & 16x & x4 & 8x & 16x & x4 & 8x & 16x & x4 & 8x & 16x \\ \hline
% 		GF \cite{he2012guided} &3.24&4.36&6.79&5.84&7.86&12.41&4.18&5.34&8.02 \\
% 		FGF \cite{wu2018fgf} & 1.94&3.36&5.81&3.21&5.92&10.45&2.45&4.42&7.26  \\
%             SVLRM \cite{pan2019spatially}&1.18&2.43&5.33&1.82&3.67&7.87&1.04&2.51&6.15&1.24&2.19\\
% 		DKN \cite{kim2021deformable} &1.23 &2.12 &4.24 &1.62 &3.26 &6.51 &0.96 &2.16 &5.11 &1.30 &1.96 &3.42 \\ 
% 		CUNet \cite{deng2020cunet} &  1.28 &2.40 &4.33 &2.22 &4.02 &6.78 &1.05 &2.48 &4.99 &1.28 &2.13 &3.45\\ 
%             DAGF \cite{zhong2021dagif} &1.28 & 2.66 & 3.80 & 2.66 & 4.97& 7.19& 1.26& 2.60& 4.77&&& \\
%         \hline
%         DCTNet\cite{zhao2022dct} &1.19 &2.35 &4.76 &1.83 &3.74 &7.16 &0.96 & 2.33 &5.38 &1.23 &2.12 &3.63\\
%         GraphSR \cite{de2022graphsr}& 1.11&2.12 &4.43 &1.79 &3.17 &6.02 &0.92 &2.05 &5.15 &1.30 &1.83 &3.12\\
%         % MADUNet \cite{madunet} &1.15 &1.69 &3.23 &1.51 &3.02 &6.23 &0.90 &1.74 &3.86\\
% 		% NAFNet \cite{chen2022nafnet} & \underline{23.73}  & \underline{0.837}  & \underline{0.126}  & \underline{34.16}  & \underline{0.909}  & \textbf{0.059}  & 30.86  &  \underline{0.908}  & \underline{0.082}   \\
% 		\hline
% 		GIRNet (Ours) &\underline{}{1.13} & \textbf{1.99} &\textbf{4.03} &\textbf{1.57} &\textbf{2.96} &\textbf{5.66} &\textbf{0.86 }& \textbf{1.95}& \textbf{4.81}&1.21&1.92&3.18  \\ \hline
% 	\end{tabular}
% 	% \label{tab:fusion}
% 	% \vspace{-2mm}
% \end{table*}

\begin{table}[!ht]
\footnotesize
\setlength\tabcolsep{3pt}
	\centering
	% \setlength{\abovecaptionskip}{0.1cm}
	\caption{The average quantitative results on the WorldView-III dataset}

	\begin{tabular}{ccccccc}
         \toprule
		\hline
		Methods & PSNR$\uparrow$  &SSIM$\uparrow$ & SAM$\downarrow$ & ERGAS$\downarrow$ & SCC$\uparrow$ & Q$\uparrow$\\ 
		\hline
		GF \cite{he2012guided} & 27.78 & 0.805 & 0.125 & 6.542 & 0.893 & 0.497  \\
		FGF \cite{wu2018fgf} & 32.49	&0.920	&0.086	&3.971	&0.947	&0.722\\
            SVLRM \cite{pan2019spatially}&32.99&0.944	&0.092	&3.572	&0.959	&0.755 \\
		DKN \cite{kim2021deformable} & 27.46 &0.742 & 0.107 & 6.861 & 0.841 & 0.418 \\ 
		CUNet \cite{deng2020cunet} & 32.46	&0.927	&0.101	&3.993	&0.949	&0.736\\ 
        DAGF \cite{zhong2021dagif} & 31.57 & 0.886&0.117&4.444&0.937&0.684\\
        % CDDFuse \cite{zhao2023cddfuse} \\
        \hline
      LAGConv \cite{jin2022lagconv} & \underline{37.12} & \underline{0.972}	& \underline{0.053}	& \underline{2.264}	& \underline{0.980} &	\underline{0.823}\\
      PANNet\cite{yang2017pannet} &32.47	&0.913	&0.097	&3.927	&0.951	&0.724\\
      GPPNN \cite{xu2021gppnn} & 35.55 &	0.962	&0.065	& 2.719 &	0.973	& 0.794\\
        MADUNet \cite{madunet} & \underline{37.12}	&0.971	&0.054	&2.267	&\textbf{0.981}	& \underline{0.823} \\
        % PGCU \cite{zhu2023probability} \\
            \hline
    GIRNet (Ours) & \textbf{37.30} &	\textbf{0.973}	&\textbf{0.052}	&\textbf{2.215}	&\textbf{0.981}	& \textbf{0.830} \\ \hline
	\end{tabular}
	\label{tab:pan}
	% \vspace{-2mm}
\end{table}


\begin{table}[!ht] \footnotesize
	\centering
	\setlength{\abovecaptionskip}{0.1cm}
	\caption{Mean and Standard Deviation of Four Metrics on Multi-Focus Image Fusion on the REALMFF and Lytro Dataset}
	\begin{tabular}{cccccc}
		\toprule
		\multirow{2}{*}{Methods}& \multicolumn{3}{c}{RealMFF} & \multicolumn{2}{c}{Lytro} \\ 
		\cmidrule(lr){2-4}
            \cmidrule(lr){5-6}
		\hline
         ~ & PSNR$\uparrow$  &SSIM$\uparrow$ & LPIPS$\downarrow$ & Q$_{MI}$$\uparrow$ & Q$_{S}$$\uparrow$ \\
            \hline
		GF \cite{he2012guided} &31.88&  0.918 & 0.098 & 1.8262 & 0.8408 \\
		FGF \cite{wu2018fgf} & 37.34 & 0.967 & \textbf{0.008} & 1.8675 & 0.8507 \\
            SVLRM \cite{pan2019spatially}&36.79& 0.975 & 0.014 & 1.8873 & \underline{0.8521} \\
		DKN \cite{kim2021deformable} & 34.22& 0.942 & 0.080 & 1.3742 & 0.8386\\ 
		CUNet \cite{deng2020cunet} & \underline{38.68} & 0.975 & 0.011 &1.8614 & 0.8410 \\ 
            DAGF \cite{zhong2021dagif} & 37.69 & 0.975 & 0.015 & 1.8961 & 0.8414 \\
            % CDDFuse \cite{zhao2023cddfuse} \\
            \hline
		IFCNN \cite{liu2017multi} & 31.61 &0.914 & 0.034 & 1.5769 & 0.7874\\
            SMFUSE \cite{ma2021smfuse} &38.54 & \underline{0.977} & 0.019 & 1.8687 & 0.8404 \\
            % U2Fusion \cite{}\\
            U2Fusion \cite{xu2020fusiondn} & 35.76 &0.972 & 0.047 & 1.8734 & 0.8318 \\
            ZMFF \cite{hu2023zmff} &34.88 & 0.956 & 0.028 & \underline{1.8874} & 0.8365  \\
            \hline
            GIRNet (Ours) & \textbf{39.71}&	\textbf{0.986} & \underline{0.009} & \textbf{1.9160} & \textbf{0.8545} \\ \hline
	\end{tabular}
	\label{tab:mfif}
	% \vspace{-2mm}
\end{table}

\begin{figure*}[t]
	\setlength{\abovecaptionskip}{0.2cm}
	\centering
	% \fbox{\rule{0pt}{2in} \rule{0.9\linewidth}{0pt}}
	\includegraphics[width=1\linewidth]{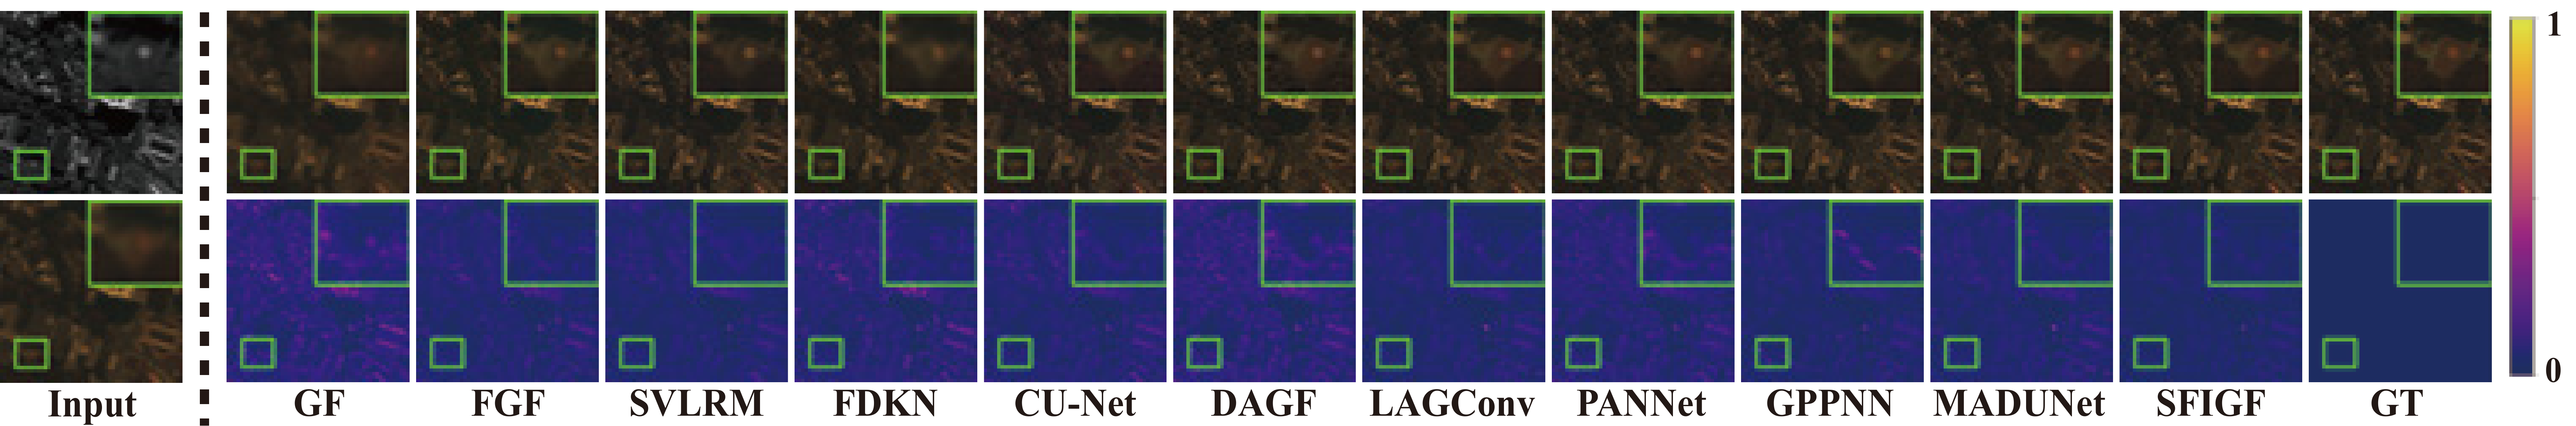}
	%\vspace{-0.5cm}
	\caption{ Visual comparison of competed methods on the WorldView-\uppercase\expandafter{\romannumeral3} of the pan-sharpening task. The bottom row refers to the corresponding RMSE maps.}
	\label{fig:pan}
	\vspace{-0.5cm}
\end{figure*}



\subsection{GIRNet for pan-sharpening}
As mentioned before, the pan-sharpening problem focuses on restoring an HRMS image $Q_{out} \in \mathbb{R} ^ {h\times w \times C}$ from an LRMS image $P \in \mathbb{R} ^ {H\times W \times C}$ with the help of an HR pan image $I \in \mathbb{R} ^ {H\times W \times 1}$, where $h<H$ and $w<W$ and the channel number $C$ is varied according to datasets, which is 8 in our experiments. Similar to GDSR, the LRMS image P can be first pre-upsampled with spatial size $H\times W$. In this application, we train our GIRNet in a supervised way with $L_1$ Loss for 3000 epochs. The initial learning rate is $1\times 10^{-4}$ and decreases as the training iterations increase.
It should be mentioned that, as demonstrated by Deng et al. \cite{jin2022lagconv}, the introduction of multi-scale structures does not improve performance for the pan-sharpening task but tends to lead to a loss of detail because of the downsampling operations. Therefore, we only use the one-scale structure in the SMFE and FeGF modules for GIRNet in this task.

% \noindent \textit{a. Experimental Settings}
\subsubsection{Datasets}
We use the WorldView-\uppercase\expandafter{\romannumeral3} dataset \cite{deng2022machine} for training and testing, where the LRMS images have 8 channels and are generated by bicubic downsampling with scale 4.
\subsubsection{Competeting Methods and evalutation metrics.}
Similar to the GDSR experiments, we consider both general-purpose GIR methods and specialized methods. Specifically, we compare our method with the same set of general-purpose methods mentioned in Sec.IV-A-a-2), and four methods that represent the state-of-the-art for the pan-sharpening task, including LAGConv \cite{jin2022lagconv}, PANNet \cite{yang2017pannet}, GPPNN \cite{xu2021gppnn}, and MADUNet \cite{madunet}.

To comprehensively evaluate the performance of each competing method, we adopt six quality assessment metrics in this task. Among them, the peak signal-to-noise ratio (PSNR) and structural similarity (SSIM) indices are commonly used image quality assessment metrics that measure pixel-level error and structural fidelity; the spectral angle mapper (SAM) \cite{yuhas1992discrimination} assessed spectral similarity for hyperspectral images (HSIs) without regard to intensity scaling; the relative dimensionless global error in synthesis (ERGAS) and correlation coefficient (SCC) captured error magnitudes across spectral bands for HSIs; and the Q index \cite{vivone2014critical} evaluated image quality {\color{red} holistically}. 

\subsubsection{ Experimental Results}

The quantitative results are shown in Table \ref{tab:pan}. It can be seen from the table that our proposed GIRNet ranks the best with respect to all the metrics, significantly outperforming the general-purpose GIR methods and also performing competitively against the state-of-the-art pan-sharpening methods. Specifically, GIRNet generates sharpened outputs with the highest PSNR and SSIM values in comparison to the  HRMS images, demonstrating its strong ability to preserve spatial information content. Besides, it also exhibits the lowest SAM and ERGAS values, indicating it most accurately retains the {\color{red} native original} spectral features and spatial patterns of the source data. Regarding SCC, GIRNet's best performance shows its effectiveness in maintaining local cross-band correlations. Furthermore, the leading score with respect to the full-reference Q index demonstrates its capacity to synthesize results most consistent with human perceptual judgments. All these quantitative results clearly verify the effectiveness of the proposed GIRNet in dealing with the pan-sharpening task.

% The qualitative results are shown in Fig.\ref{fig:pan}. With the help of Root Mean Square Error (RMSE) maps in the bottom row, it can be found that our methods have succeded in recovering the degraded details and shown outstanding performance compared with both of the generative methods and the specifically-designed pan-sharpening methods.
The qualitative results in Fig.\ref{fig:pan} provide a visual comparison of our proposed method against existing ones. As shown in the top row, our GIRNet is able to successfully reconstruct fine-scale details that were degraded in the LrMS images. The root mean square error (RMSE) maps in the bottom row provide a more easily observable validation of these qualitative findings. Specifically, the RMSE maps show that our method achieves the lowest error values, indicating its predictions most closely match the HRMS images. These results suggest our method can effectively leverage contextual information to reconstruct high-frequency details for this task.
\subsection{GIRNet for MFIF}
The MFIF task aims at fusing spatially complementary visual content
from multiple source frames exhibiting focus disparities and reconstructing an all-in-focus image. Typically in this task, two inputs depicting the same scene at near and far focal distances are fused. 
Therefore, this problem can be treated as a mutually guided image restoration, where the two input images guide each other for the final reconstruction.
Since our proposed GIRNet distinguishes the guidance image from the guided image for two input sources, we need to slightly modify it to adapt to this task. 
Specifically, we employ a dual-guidance framework, within which to operate in parallel and each GIRNet takes one image as the guidance and the other as the guided one.
Then the middle results of the two GIRNet branches are fused at the output layer to get the final reconstruction.
The whole dual framework is as follows:
\begin{gather}
    Q_{out}^1 = GIRNet_1(I_1, I_2),\\
    Q_{out}^2 = GIRNet_2(I_2, I_1),\\
    Q_{out} = Conv(Cat(Q_{out}^1, Q_{out}^2))
\end{gather}
where $I_1, I_2 \in \mathbb{R}^{H\times W\times3}$ refers to inputs captured with near and far views. Besides, as mentioned in Sec.\ref{sec:rlmff}, the MFIF task is commonly formulated in an unsupervised manner to meet practical requirements, and thus we utilize two unsupervised losses for network training without relying on ground truth images:
\begin{gather}
    L_2 = s_1\|Q_{out}-I_1\|_2^2 + s_{2}\|Q_{out}-I_2\|_2^2,\\
    L_{grad} = s_{1}\|\nabla Q_{out}-\nabla I_1\|_2^2 + s_{2}\|\nabla Q_{out}-\nabla I_2\|_2^2,\\
    L = L_2 + L_{grad},
\end{gather}
 {\color{red} where $s_{1} = sgn(HF(I_1)-min(HF(I_1), HF(I_2)))$, $s_{2} = 1 - s_{1}$. $\nabla$ refers to the gradient operator. $HF(\cdot)$ refers to the high-frequency contents of the image, calculated by the Gaussian filtering kernel.} In the MFIF application, we train the GIRNet for 200 epochs whose batch size is 16 and the initial learning rate is $1x10^{-4}$.

% \noindent \textit{a. Experimental Settings}
\subsubsection{Datasets}
We evaluate the effectiveness of our method on the Real-MFF dataset \cite{zhang2020real}, which consists of various natural multi-focus images with ground truth, generated by light field images.
We use the first 650 pairs of images for training and the last 60 pairs of images for testing. 
Besides, we conduct an evaluation on the widely used real-world Lytro dataset \cite{nejati2015multi} to show our generalization. It contains 20 pairs of multi-focus images obtained by the light-field camera with a size of 520 × 520.
% It is worth noting that obtaining ground truth images for reference is challenging to achieve in practice. As such, our proposed model is trained in an unsupervised fashion, without directly supervised learning from fused ground truths.

\subsubsection{Competeting Methods and evaluation metrics}
In addition to the six general-purpose GIR methods used before, four state-of-the-art DL-based fusion methods were adopted for evaluation, including IFCNN \cite{liu2017multi}, SMFUSE \cite{ma2021smfuse}, U2Fusion \cite{xu2020fusiondn}, and ZMFF \cite{hu2023zmff}. All the competing methods are trained in an unsupervised manner or implemented in a zero-shot way, without reference to the ground truth.
To numerically evaluate the fusion results, we adopt three common image quality assessment metrics, including PSNR, SSIM, and LPIPS.
For evaluation on the non-reference dataset Lytro, we use the information theory-based metrics Q$_{MI}$ and the image structure similarity-based metric Q$_{S}$ following \cite{hu2023zmff}.

\subsubsection{Experimental Results}

The qualitative results of all competing methods are reported in Table \ref{tab:mfif}, and we can see that our GIRNet achieves the best performance among all methods, obtaining 1.03 dB improvement in PSNR and 0.009 improvement in SSIM compared with the second best ones, and takes the second place on LPIPS, showing our outstanding perceptual quality.
For the Lytro dataset, we also achieve first place among all methods, presenting that our results have the richest information extracted from source images and share highest similarity with sources based on SSIM.
These improvements demonstrate the effectiveness of our method for this task. 

% The qualitative results are shown in Fig.\ref{fig:mff}. From the bottom row, we can see that our methods succeed in combining both near and far views. We also show error maps which refer to the mean square error (MSE) distance between prediction and ground truth. The error maps show that our method can recover more accurate structures compared with both generative and specific methods even in an unsupervised way. 
The visual results presented in Fig.\ref{fig:mff} further verify the superiority of the proposed GIRNet over existing methods. Specifically, as shown in the top row, our method is able to successfully synthesize images that integrate both near-view details and far-view context. The mean square error (MSE) maps in the bottom row make this observation clearer and indicate a more accurate structural reconstruction of our method against other competing methods, with reference to the ground truth. The visual comparisons of Lytro are shown in the SM because of the space limitation.
% In comparison to both generative models and techniques designed specifically for multi-focus fusion, our method qualitatively synthesizes better-focused images and quantitatively achieves superior performance.

\begin{figure*}[t]
	\setlength{\abovecaptionskip}{0.2cm}
	\centering
	% \fbox{\rule{0pt}{2in} \rule{0.9\linewidth}{0pt}}
	\includegraphics[width=1\linewidth]{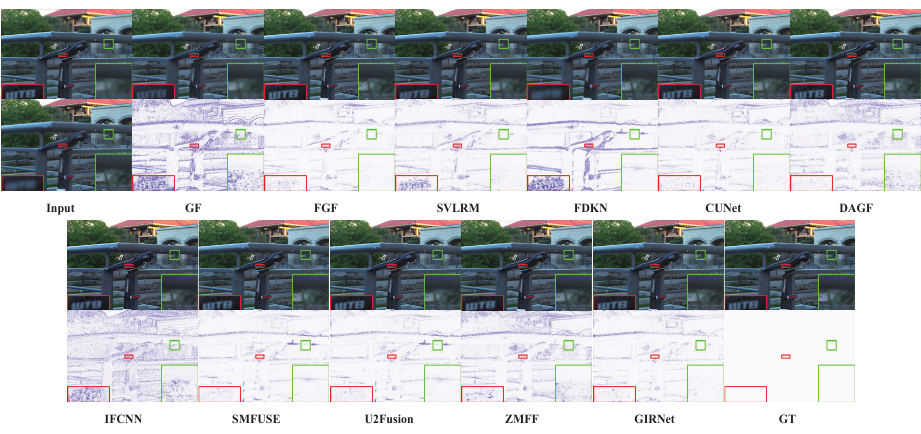}
	%\vspace{-0.5cm}
	\caption{Visual comparison of competed methods on the Real-MFF dataset of the MFIF task. The bottom row refers to the corresponding error maps.}
	\label{fig:mff}
	% \vspace{-0.5cm}
\end{figure*}


% \begin{figure*}[t]
% 	\centering
%  \captionsetup[subfloat]{labelsep=none,format=plain,labelformat=empty}
% 	\setlength{\abovecaptionskip}{0.1cm}
% 	\subfloat[RAW ]{\includegraphics[width=0.14\linewidth]{./results/lrie/inp.pdf}}
% 	\subfloat[Bicubic ]{ \includegraphics[width=0.14\linewidth]{./results/lrie/bi.pdf}}
% 	\subfloat[GF]{ \includegraphics[width=0.14\linewidth]{./results/lrie/gf.pdf}} 
% 	\subfloat[FGF ]{	\includegraphics[width=0.14\linewidth]{./results/lrie/fgf.pdf}}
% 	\subfloat[SVLRM ]{ \includegraphics[width=0.14\linewidth]{./results/lrie/svlrm.pdf}}
% 	\subfloat[FDKN]{	\includegraphics[width=0.14\linewidth]{./results/lrie/fdkn.pdf}} 
%  \subfloat[CUNet \cite{deng2020cunet}]{	\includegraphics[width=0.14\linewidth]{./results/lrie/fdkn.pdf}} 
%  \\
%  \vspace{-3mm}
%  \subfloat[DAGF ]{	\includegraphics[width=0.14\linewidth]{./results/lrie/dagf.pdf}}
%  \subfloat[SID]{	\includegraphics[width=0.14\linewidth]{./results/lrie/sid.pdf}}
%  \subfloat[SGN]{	\includegraphics[width=0.14\linewidth]{./results/lrie/sgn.pdf}}
%  \subfloat[EEMEFN]{	\includegraphics[width=0.14\linewidth]{./results/lrie/eemefn.pdf}}
%  \subfloat[DBLE]{	\includegraphics[width=0.14\linewidth]{./results/lrie/dble.pdf}}
%  \subfloat[GIRNet]{	\includegraphics[width=0.14\linewidth]{./results/lrie/girnet.pdf}}
%   \subfloat[GT]{	\includegraphics[width=0.14\linewidth]{./results/lrie/gt.pdf}}
% 	\caption{Visual comparison of competed methods on the SID-Sony dataset of the LRIE task.}
% 	\vspace{-0.5cm}
% 	\label{fig:lrie} 
% \end{figure*}


\subsection{GIRNet for guided LRIE}
% The goal of LRIE is to enhance the quality of the RAW image captured under extremely low-light conditions, typically through the deep image signal processing (ISP) pipeline \cite{chen2018learning}. Currently, a widely used and effective strategy for dealing with this task is to make use of guide information, either self-generated \cite{zhu2020eemefn} or auxiliary \cite{dong2022abandoning}. Therefore, our GIRNet can be naturally applied to the LRIE task, by treating it as a  GIR problem. To distinguish whether the guidance is self-generated or auxiliary, we consider two sets of applications here. The first is pure LIRE, i.e., one can only use the information of the RAW image itself, which means that the guidance can only be self-generated; the second is the guided LIRE, in which one can use auxiliary guidance information, e.g., the red flashlight image \cite{lamba2021red} or the monochrome image \cite{dong2022abandoning}.


Following the work by Xiong et al. \cite{xiong2021mffnet} and Dong et al. \cite{dong2022abandoning}, which respectively used the red flashlight image and the monochrome image as the guidance for low-light image enhancement of RAW image, we consider two scenarios of guided low-light image enhancement tasks: (1) RAW image with red flashlight RAW guidance and (2) RAW image with monochrome RAW guidance. 

\subsubsection{Datasets}
For the first task, we synthesize paired RAW/red flashlight dataset from the Sony dataset of the SID dataset \cite{chen2018learning}, which is constructed by extremely low-light RAW images. Images in the Sony dataset are captured by the Sony $\alpha$7S \uppercase\expandafter{\romannumeral2} Bayer sensor with the size $4256 \times 2848 \times 1$.
 For the second, we adopt the Mono-Colored RAW (MCR) paired dataset collected by Dong et al. \cite{dong2022abandoning}. All the input RAW images are packed into 4 channels before being inputted into networks following \cite{chen2018learning}.

\subsubsection{Competing methods and evaluation metrics} 
In addition to the six general-purpose GIR methods, we consider two recently proposed guided LRIE methods, i.e., MFFNet \cite{xiong2021mffnet} and DBLE \cite{dong2022abandoning}. We use the same sets of evaluation metrics as in the LIRE experiments.
Four metrics, including PSNR, SSIM, LPIPS \cite{zhang2018lpips} and Delta E ($\triangle E^{*}$) \cite{backhaus2011color}, are adopted for quantitative evaluation. Among these metrics, PSNR and SSIM are general image quality assessment metrics, LPIPS is a deep feature-based %\footnote{We employ the AlexNet as the feature extractor.} 
metric aiming at assessing the perceptual quality of an image with a reference image, $\triangle E^{*}$ is a metric to measure the color distortion.

\subsubsection{ Experimental Results}
The quantitative evaluation results for all comparison methods are reported in Table \ref{tab:glrie}. It can be seen that our proposed GIRNet model achieves superior performance across all evaluated metrics compared with other competing approaches, which shows the outstanding abilities of our method in reconstructing textual and contextual information and overcoming color biases.

{\color{red} Fig. \ref{fig:red}-\ref{fig:mcr} show example qualitative results as well as the corresponding error maps. It can be visually observed from the error maps that our method produces results with fewer residuals compared with the ground truths.}

% As demonstrated in the error maps for images corrupted with both noise and color casts, GIRNet restores images with finer edges and more accurate textures. This validates the robustness of our approach against common image artifacts like noise and color distortions.

 
% \begin{table}[!ht]
% 	\small
% 	\centering
%  \setlength{\abovecaptionskip}{0.0cm}
% 	\caption{Quantitative results of all competing LRIE methods on the SID dataset. The best and second-best results are highlighted in bold and with an underline, respectively.\label{tab:sid} }
% 	\begin{tabular}{ccccc}
% 		\toprule
% 		Methods & PSNR$\uparrow$ & SSIM$\uparrow$ & LPIPS$\downarrow$ &$\triangle \textit{E}^{*}\downarrow$ \\ \hline
% 		GF \cite{he2010guided}   & 16.03 & 0.519 & 0.410  & 18.76        \\
% 		FGF \cite{wu2018fgf}   & 28.84 & 0.768 & 0.310 & 5.035    \\
%             SVLRM \cite{pan2019spatially} &28.56 & 0.763 & 0.260 & 5.587  \\
%             DKN \cite{kim2021deformable} & 25.39 & 0.692&0.362&6.848 \\
%             CUNET \cite{deng2020cunet} & 28.37& 0.774 & 0.280 & 5.579 \\
%              DAGF \cite{zhong2021dagif} & 30.07&	0.800 &	0.245 &	4.500 \\
%              % CDDFuse \cite{zhao2023cddfuse} \\
%             \hline
% 		SID \cite{chen2018learning}     & 29.57 & 0.799 & \underline{0.246} & 4.901      \\
%         % LRDE \cite{xu2020lrde}  & 29.66 & 0.794 & 0.253  & 4.689 \\
% 		SGN  \cite{gu2019sgn} & 29.45 & 0.796 & 0.248 & 4.936    \\
% 		EEMEFN \cite{zhu2020eemefn}   & \underline{30.08} & \underline{0.801} & 0.247 & \underline{4.662}    \\
% 		% RED \cite{lamba2021red}    & 28.66 & 0.790  & 0.312 & 20.17   \\
% 		DBLE \cite{dong2022abandoning} & 29.70 & 0.796 & 0.247 & 4.759      \\
       
%         % DNF \cite{jin2023dnf} &28.71 &  0.726  & 0.391 & &30.62&0.797&0.343 & & 2.800 & 57.00\\
%         \hline
%   GIRNet (Ours)   & \textbf{30.27} & \textbf{0.804} &\textbf{0.245} & \textbf{4.522}   \\\hline
% 	\end{tabular}
% 	\vspace{-4mm}
% \end{table}


\begin{table*}[!ht]\small
	\centering
	\setlength{\abovecaptionskip}{0.1cm}
	\caption{Quantitative results of all competing methods on guided LIE tasks. The best and second-best results are highlighted in bold and with an underline, respectively.}
	\begin{tabular}{ccccccccc}
		\toprule
		\multirow{2}{*}{Methods}&  \multicolumn{4}{c}{Sony (RAW+Red)} &  \multicolumn{4}{c}{MCR (RAW+Mono)} \\ 
  % \multirow{2}{*}{Methods}& \multicolumn{3}{c}{Middlebury} & \multicolumn{3}{c}{NYU V2} &  \multicolumn{3}{c}{Lu} & \multicolumn{3}{c}{Average}
            \cmidrule(lr){2-5}
            \cmidrule(lr){6-9}
		% \hline
		~ & PSNR $\uparrow$ & SSIM $\uparrow$ & LPIPS $\downarrow$ & $\triangle E^{*}\downarrow$ & PSNR$\uparrow$ & SSIM$\uparrow$ & LPIPS$\downarrow$ & $\triangle E^{*}\downarrow$   \\ \hline
		GF \cite{he2012guided} & 16.25 & 0.674 & 0.328 & 18.61 & 16.04 & 0.697 & 0.405 & 14.47  \\
		FGF \cite{wu2018fgf}  & 30.80  & 0.857  & 0.129  & 4.453 & 23.93  & 0.830  & 0.176 & 6.660  \\
            SVLRM \cite{pan2019spatially}&32.34 & 0.890 & 0.075 & 3.857 & 25.83	& 0.879& 0.103 & 5.758 \\
		DKN \cite{kim2021deformable} & 26.68  & 0.720  & 0.232 & 6.467 & 23.43  & 0.838  & 0.151  & 7.528 \\ 
		CUNet \cite{deng2020cunet} & 30.99  & 0.881  & 0.091 & 4.290 & 19.70  & 0.673  &  0.257 & 11.55 \\ 
            DAGF \cite{zhong2021dagif} & 27.96 &0.887 &0.090 & 5.592 & 26.67 &0.873&0.126&5.241\\
            % CDDFuse \cite{zhao2023cddfuse} \\
		\hline
		DBLE \cite{dong2022abandoning}  & \underline{33.36}  & \underline{0.893} & \underline{0.075}  & \underline{3.622} & \underline{31.69}  & \underline{0.908}  & \underline{0.082} &\underline{3.133}  \\ 
		MFFNet \cite{xiong2021mffnet}  & 30.99  & 0.876  & 0.101 & 4.440 & 28.62  & 0.902  & 0.096 & 4.316  \\
		% NAFNet \cite{chen2022nafnet} & \underline{23.73}  & \underline{0.837}  & \underline{0.126}  & \underline{34.16}  & \underline{0.909}  & \textbf{0.059}  & 30.86  &  \underline{0.908}  & \underline{0.082}   \\
		\hline
		GIRNet (Ours) &\textbf{34.25}  & \textbf{0.902}  & \textbf{0.067} & \textbf{3.304} & \textbf{32.11} 	&\textbf{0.925} &	\textbf{0.065} &	\textbf{3.077 }  \\ \hline
	\end{tabular}
	\label{tab:glrie}
	\vspace{-2mm}
\end{table*}


\begin{figure*}[t]
	\setlength{\abovecaptionskip}{0.2cm}
	\centering
	% \fbox{\rule{0pt}{2in} \rule{0.9\linewidth}{0pt}}
	\includegraphics[width=1\linewidth]{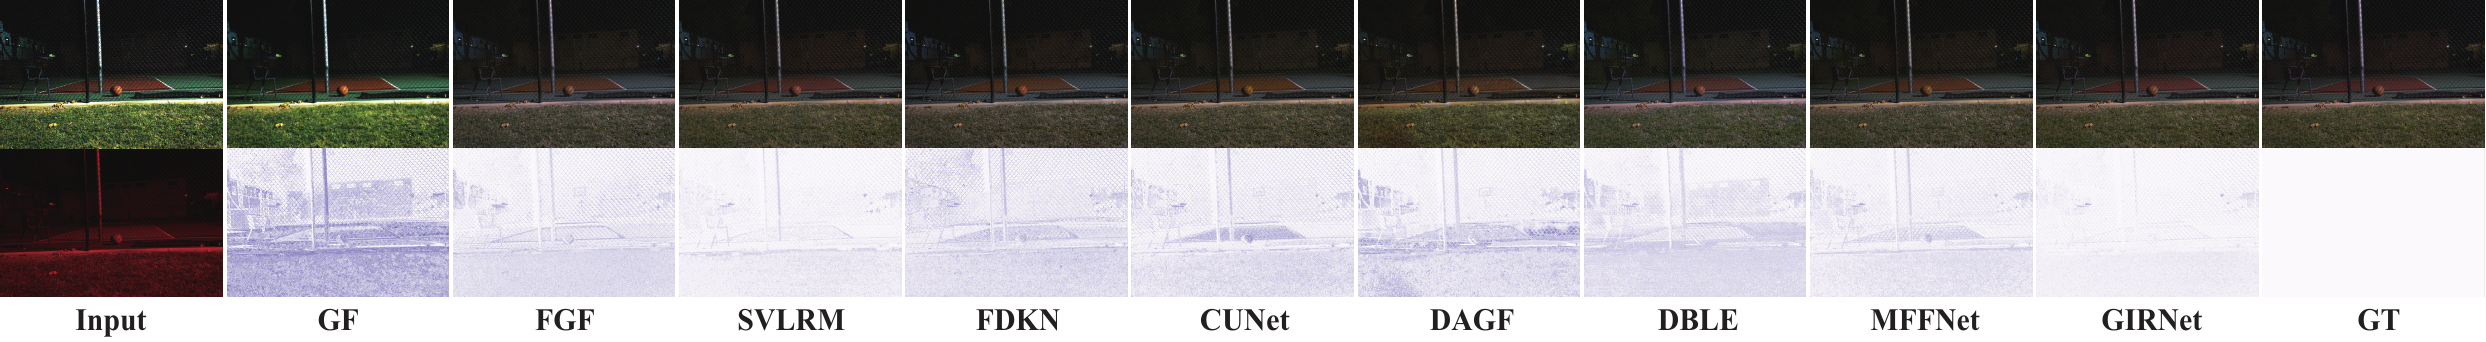}
	%\vspace{-0.5cm}
	\caption{Visual comparison of competed methods on the SID-Sony dataset of the red-guided LRIE task. The bottom row refers to the corresponding error maps.}
	\label{fig:red}
	% \vspace{-0.5cm}
\end{figure*}

\begin{figure*}[t]
	\setlength{\abovecaptionskip}{0.2cm}
	\centering
	% \fbox{\rule{0pt}{2in} \rule{0.9\linewidth}{0pt}}
	\includegraphics[width=1\linewidth]{./results/mcr/mcr_48.pdf}
	%\vspace{-0.5cm}
	\caption{ Visual comparison of competed methods on the MCR dataset of the mono-guided LRIE task. The bottom row refers to the corresponding error maps.}
	\label{fig:mcr}
	% \vspace{-0.5cm}
\end{figure*}

%%%%%%%%%%%%%%%%%%%%%%%%%%%%%%%%%%%%%%%%%%%%%%%%%%%%%%%%%%%%%%%%%%%%%%%%%%%%%%%%%%%%%%%%

\begin{figure*}[t]
	\setlength{\abovecaptionskip}{0.2cm}
	\centering
	% \fbox{\rule{0pt}{2in} \rule{0.9\linewidth}{0pt}}
	\includegraphics[width=1\linewidth]{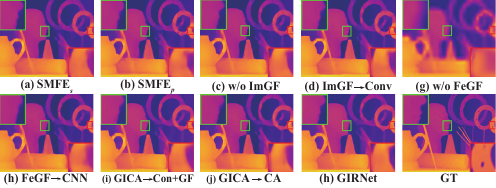}
	%\vspace{-0.5cm}
	\caption{ Visual comparison of competed methods on the MCR dataset of the mono-guided LRIE task. The bottom row refers to the corresponding error maps.}
	\label{fig:ablation}
	% \vspace{-0.5cm}
\end{figure*}
\begin{table}[t]
\footnotesize
	\centering
	% \setlength{\abovecaptionskip}
	\caption{RMSE results on the 16x GDSR task of the ablation study.\label{tab:ablation} }
	% \begin{adjustbox}{width=0.95\linewidth, center}
		\begin{tabular}{l cccc}
			\hline 
			Settings & Middlebury &NYU V2 &Lu &Average \\ \hline
                (a) SMFE$_p$   &  3.53 &5.89 &4.57& 	4.63  \\ 
                (b) SMFE$_s$  & 3.61 & 6.10 &4.45 &4.75 \\
                \hline
                (c) only FeGF (w/o ImGF)  &3.54 &	5.95 	&4.48 & 4.66 \\ 
                (d) ImGF $\rightarrow$ Conv & 3.52 	& 5.89 &4.53 & 4.65 \\
                (e) SVLRM & 5.33 & 7.87 & 6.15 & 6.45\\
                (f) SVLRM with ImGF & 4.79 & 7.28 & 5.57 & 5.88 \\
                \hline
                (g) only ImGF (w/o FeGF) & 6.36 & 11.2 &7.22 & 7.35 \\
                 (h) FeGF $\rightarrow$ CNN &3.63 	& 6.11 	&4.62 	& 4.79 \\
                 (i) GICA $\rightarrow$ Conv & 3.48 &	6.12 & 4.29 & 4.74 \\
                 (j) GICA $\rightarrow$ CA & 3.70 &	6.28 & 4.63 & 4.87 \\

                 
                  % ImGF $\rightarrow$ SVLRM \\
			% only ImGF$_{l}$ & & & & & 0.076 & 18.97 \\ 
			\hline
			(k) GIRNet (Ours) & \textbf{3.38} &	\textbf{5.75} 	& \textbf{4.38} & \textbf{4.57 }\\\hline
		\end{tabular}
	% \end{adjustbox}
	% \vspace{-7mm}
\end{table}

 \subsection{Effectiveness of modules in GIRNet \label{sec:ablation}}
In this subsection, we conduct experiments on the 16x GDSR task to verify the necessity and effectiveness of key modules, including SMFE, ImGF, and FeGF in the proposed GIRNet. The overall results are summarized in Tabel \ref{tab:ablation}, and shown in Fig. \ref{fig:ablation}. 



\begin{figure}[t]
	\setlength{\abovecaptionskip}{0.2cm}
	\centering
	% \fbox{\rule{0pt}{2in} \rule{0.9\linewidth}{0pt}}
	\includegraphics[width=1\linewidth]{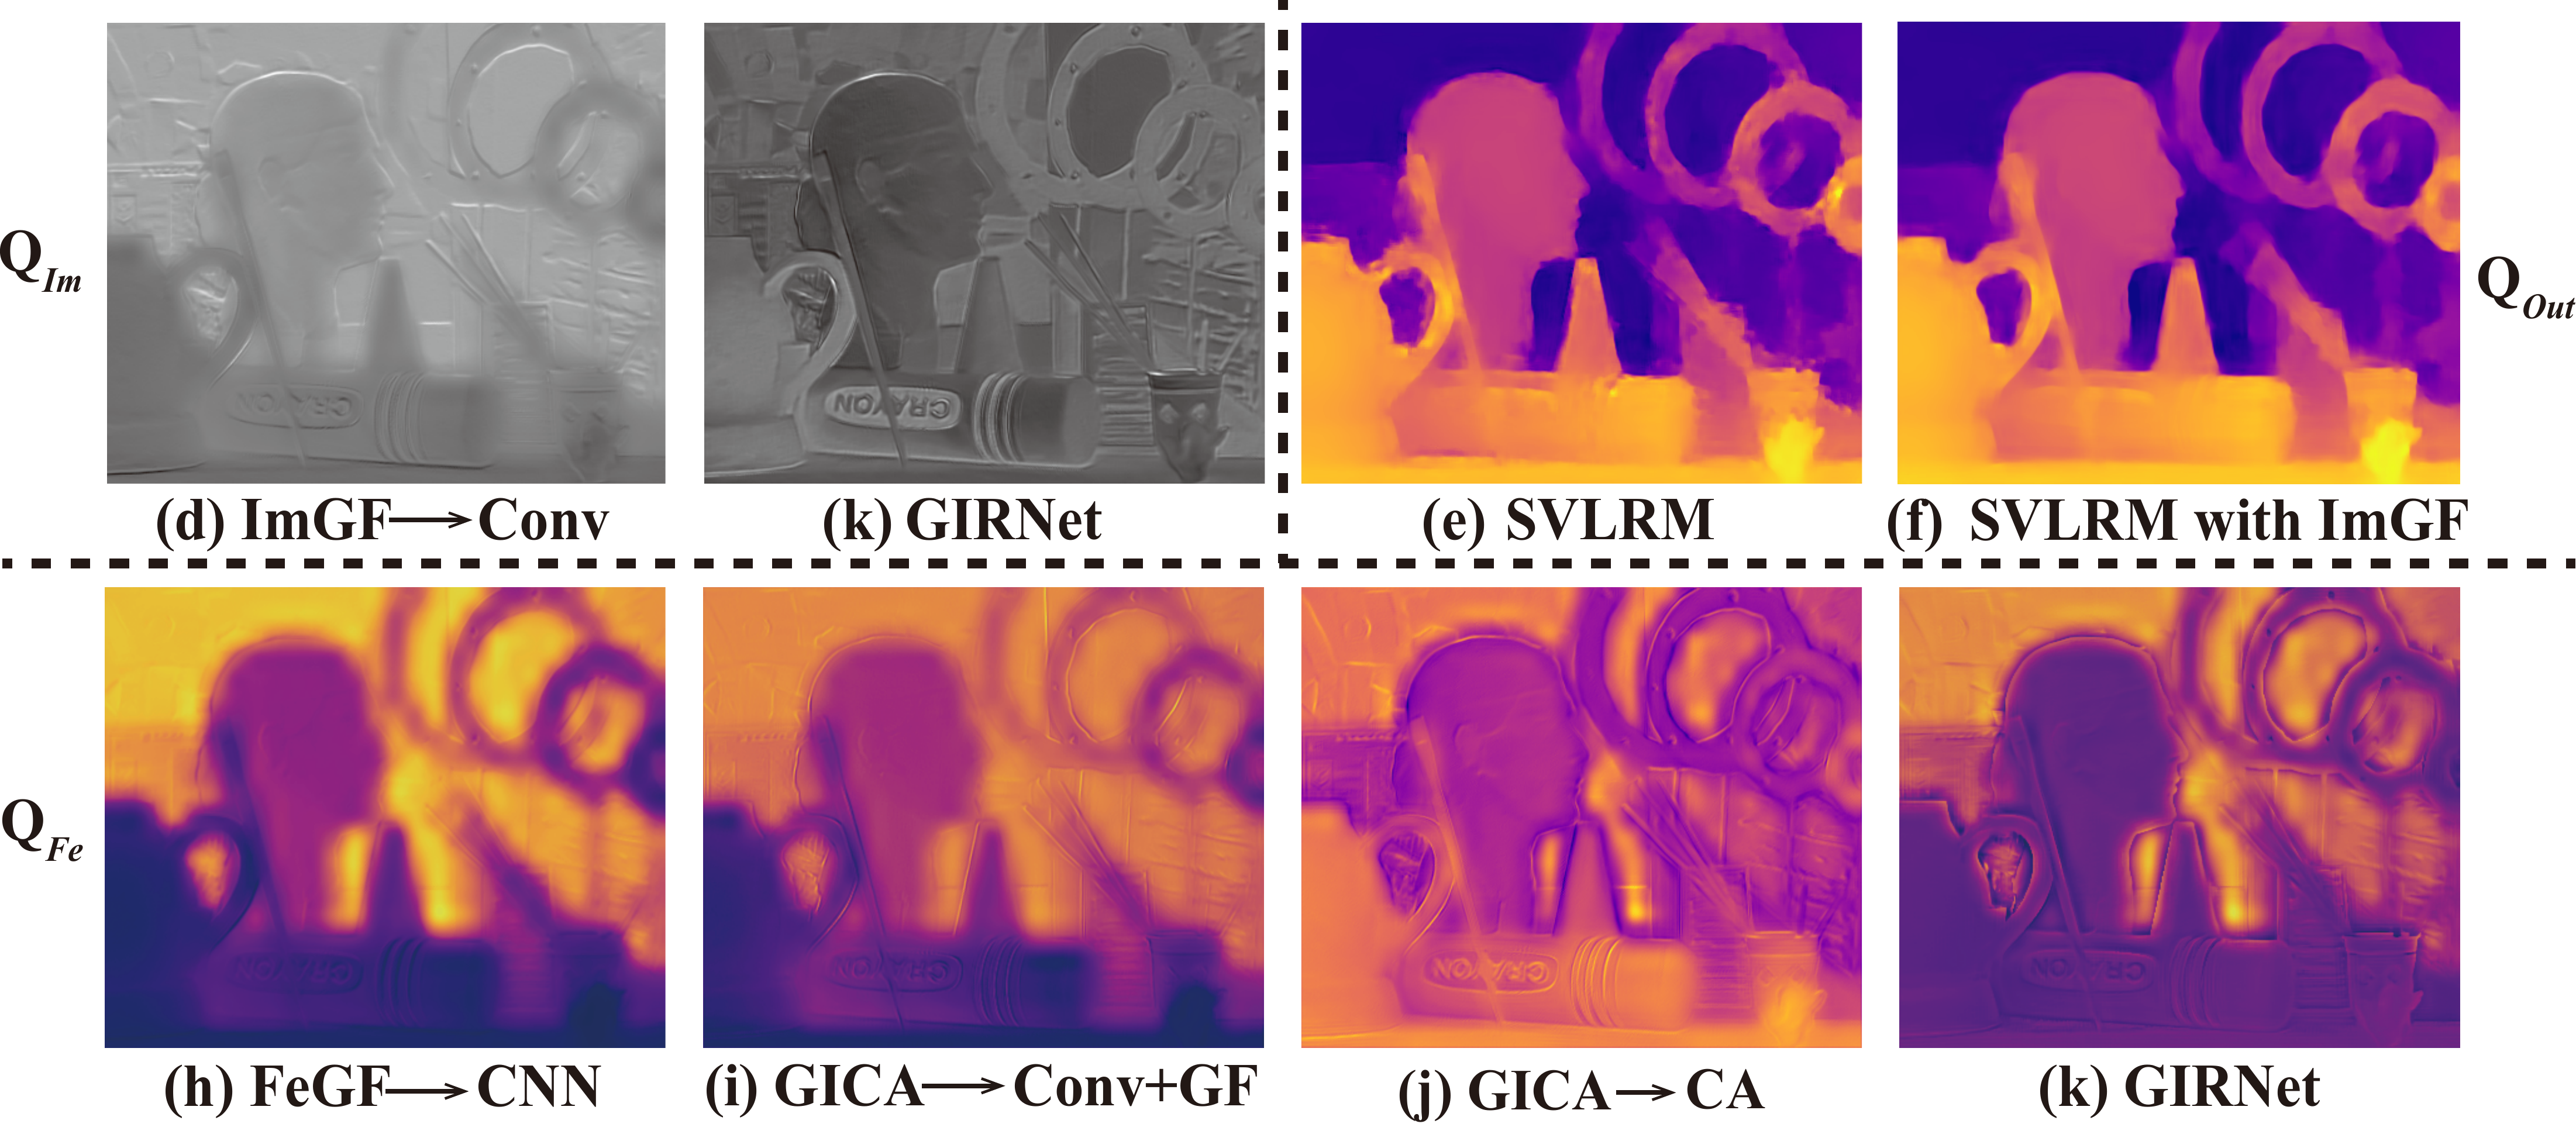}
	%\vspace{-0.5cm}
	\caption{ Visual comparison of competed methods on the MCR dataset of the mono-guided LRIE task. The bottom row refers to the corresponding error maps.}
	\label{fig:abqq}
	% \vspace{-0.5cm}
\end{figure}


\subsubsection{Effectiveness of the SMFE module}
% We conduct experiments to verify the necessity of the two key modules, ImGF and FeGF, in our GIRNet. These two modules are responsible for fusion in image and feature domains, respectively, and we show that both of them play important roles.

We first conduct ablation experiments to evaluate the effectiveness of our proposed SMFE module in cooperatively extracting shared and private information from source images. Specifically, we compared our model against two baselines\textemdash a \textbf{shared} setting where source images are directly concatenated as input, which is denoted as \textit{SMFE$_{s}$},  and a \textbf{private} setting where each source is processed independently by separate feature extractors, which is denoted as \textit{SMFE$_{p}$}.
For the shared baseline, the concatenated inputs were passed through a feature extractor with NAF blocks as the basic module, retaining the skip connections. In the private setting, each source was processed individually by isolated NAF feature extractors.

As shown in Table \ref{tab:ablation}, both settings exhibited decreased performance quantitatively compared to our full model across all datasets.
Qualitatively, visualization of results in Fig. \ref{fig:ablation} revealed that our SMFE module was able to better capture fine-grained details like object edges and produce images with a more even appearance, while the compared settings exhibited degraded ability in edge refinement and surface reconstruction. 
Furthermore, we visualize the extracted features by different approaches in Fig. \ref{fig:absmfe}. It can be observed that, compared with GIRNet, both the $i_ts$ and $p_ts$ of \textit{SMFE$_{p}$}, which are extracted respectively,  are unable to extract the necessary structural contents without the Mutual information extraction. In contrast, employing a completely shared SMFE to extract $i_{ts}$ and $p_{ts}$ preserves similar structural information across the two representations while also retaining unexpected texture details. 
% This evaluation empirically validates the effectiveness of our proposed module in disentangling shared and private representations from multiple related inputs, outperforming alternative designs that do not separate modality-specific information. It demonstrates the importance of modeling both shared and private content for the task of multi-modal image fusion.

\subsubsection{Effectiveness of the FeGF module}
We began by investigating a model utilizing only the ImGF module to demonstrate the importance of the FeGF module. Not surprisingly, without feature restoration capabilities, the performance degraded substantially as shown in (g) Fig.\ref{fig:ablation} and Table \ref{tab:ablation}.
Additionally, to further evaluate the impact of incorporating the GF mechanism, we conducted an ablation experiment by completely replacing the whole FeGF module with a series of CNN layers. The results are reported quantitatively in Table \ref{tab:ablation} (h) and qualitatively depicted in Figure \ref{fig:ablation} (h), and both of them indicate performance degradation with respect to the full GIRNet model, validating the importance of the GF mechanism.
For deeper insight, we visualize the feature domain restoration output \textit{Q$_{Fe}$} with and without GF in Figure \ref{fig:abqq} (k) and (h). The reconstruction exhibits unclear edges when GF cues are not provided to guide the restoration, highlighting the role of the GF mechanism in preserving structures from the guidance features $i_ts$.

Since the GF mechanism is achieved in our model via the proposed GICA block, we want to further analyze its necessity. In specific, we conduct another ablation test of replacing the CA and SA blocks with standard CNN layers while maintaining the overall GF design. This setting keeps the GF mechanism by $q_t = A_t * i_t + b_t$, where $A_t$ and $b_t$ are learned by convolutional layers.
It can be seen from Table \ref{tab:ablation} that the quantitative performance is dropped by this setting. In addition, Fig. \ref{fig:abqq} and \ref{fig:ablation} (i) provide the visual results. It can be observed that the details are less clear compared with GIRNet due to the abilities of SA and CA to capture long-range dependencies, which is beneficial for reconstructing information degraded by downsampling operations.
When comparing (h) and (i), it can be seen that completely lacking the guidance of GF by completely replacing the FeGF module with ordinary CNN layers without the GF mechanism, can result in blurrier edges. All the observations indicate that the effectiveness of our FeGF module is not only from the attention blocks but also from the introduction of the GF mechanism which helps to preserve structural information from guidance features. 
Besides, we conduct the experiment of replacing our GICA block with the original CA block. It can be seen from (j) in Table \ref{tab:ablation} and Figure \ref{tab:ablation} that both the qualitative and quantitive results are degraded. Furthermore, when compared with (i), the original CA block performs worse, since it loses the important GF mechanism without the learned residual $b$ in Eq. \ref{eq:fegf_ca}.
Combined with quantitative findings, these provide preliminary evidence that both the FeGF module and its GF-based cross-attention modules contribute favorable information fusion beyond conventional CNN designs lacking these capabilities.

\subsubsection{Effectiveness of the ImGF module}

To evaluate the effectiveness of ImGF, we first conduct an experiment without it and keep only the FeGF module.
As shown in (c) of Table \ref{tab:ablation}, removing ImGF led to degraded quantitative performance on all datasets. Qualitative results in (c) Fig.\ref{fig:ablation} further revealed deficits in this setting, that it loses fine image details and generates blurred edges. This validates that ImGF plays a crucial role in preserving the original textural information from the source images.

To further verify the effectiveness of the introduction of the GF mechanism in the ImGF module, we also conduct an experiment by replacing the ImGF module with CNN layers and observe the degraded performance both quantitatively and visually. Specifically, Fig.\ref{fig:ablation} (d) shows that the edges detected by the CNN-only model appear {\color{red}more blurry} compared to the present ImGF model. The output $Q_{Im}$ of this branch in this setting is shown in Fig. \ref{fig:abqq} (d). It can be observed that without the GF mechanism, the fused result \textit{Q$_{Im}$} suffers from loss of textual information and generates blurry edges. 
These results demonstrate that incorporating the GF into the ImGF module enhances model performance over using CNN layers alone.

{\color{red} As demonstrated in Section \ref{sec:imgf}, our proposed guided restoration module in the image domain follows more closely to the original GF mechanism compared with SVLRM \cite{pan2019spatially}. To show our effectiveness, we additionally conducted the experiment on SVLRM by replacing the inputs of its parameters learning network with our strategy. The compared quantitative results are listed in (e) and (f) in Table \ref{tab:ablation}. It can be observed that our mechanism have benefit in improving recovery performance. }

Having the supplementary compiled together with the main paper means that:
% 
\begin{itemize}
\item The supplementary can back-reference sections of the main paper, for example, we can refer to \cref{sec:intro};
\item The main paper can forward reference sub-sections within the supplementary explicitly (e.g. referring to a particular experiment); 
\item When submitted to arXiv, the supplementary will already included at the end of the paper.
\end{itemize}
% 
To split the supplementary pages from the main paper, you can use \href{https://support.apple.com/en-ca/guide/preview/prvw11793/mac#:~:text=Delete%20a%20page%20from%20a,or%20choose%20Edit%20%3E%20Delete).}{Preview (on macOS)}, \href{https://www.adobe.com/acrobat/how-to/delete-pages-from-pdf.html#:~:text=Choose%20%E2%80%9CTools%E2%80%9D%20%3E%20%E2%80%9COrganize,or%20pages%20from%20the%20file.}{Adobe Acrobat} (on all OSs), as well as \href{https://superuser.com/questions/517986/is-it-possible-to-delete-some-pages-of-a-pdf-document}{command line tools}.
